# Supplementary material for: The competing risks Cox model with and without auxiliary case covariates under weaker or no missing-at-random cause of failure
Source: arXiv:1607.08882 source file (2016-07-29)
Supplement: Supplementary file 1 [file MissingSubtypeSuppArXiv.pdf]

# Supplementary Materials for "The competing risks Cox model with and without auxiliary case covariates under weaker or no missing-at-random cause of failure"


Daniel Nevo*[1,2], Reiko Nishihara[3,4], Shuji Ogino[2,4,5] and Molin Wang[1,2]

[1]Department of Biostatistics, Harvard T.H. Chan School of Public Health
[2]Department of Epidemiology, Harvard T.H. Chan School of Public Health
[3]Department of Nutrition, Harvard School of Public Health
[4]Department of Medical Oncology, Dana-Farber Cancer Institute
[5]Division of MPE Molecular Pathological Epidemiology, Department of Pathology , Brigham and Women's Hospital and Harvard Medical School


## Web Appendix A: Asymptotic properties of proposed estimators

We present here proofs for the consistency and asymptotic normality of the maximum partial likelihood estimator with respect to $L^{\star}_{Q2}$ under $\text{MAR}_{T,\boldsymbol{X},\boldsymbol{Q}}$. The proofs for the estimator obtained from $L^{\star}_{Y}$ can be constructed in a similar manner, and assumptions about the distribution of $\boldsymbol{Q}$ with assumptions on $\pi$. Consider $\boldsymbol{\theta} = (\boldsymbol{\beta}, \boldsymbol{\psi}, \boldsymbol{\eta})$ and let $\boldsymbol{\theta}_0$ denote its true value. We denote $\pi(t, \boldsymbol{x}, \boldsymbol{q})$ ($\overline{\pi}(t, \boldsymbol{x}, \boldsymbol{q})$) for the probability of observing (not observing) the cause given event was observed and given other known data by time $t$. For convenience reasons, we take $\boldsymbol{Q}$ here to be a vector of $n_q$ continuous random variables, defined on a sample space $\Omega_{\boldsymbol{q}} \in \mathcal{R}^{n_q}$, and we let $\nu_k(\boldsymbol{q}, \boldsymbol{x}, t; \boldsymbol{\psi})$ to be its joint probability density function given $Y = k, \boldsymbol{X} = \boldsymbol{x}$ and $\tilde{T} = t$.

For any function $h(\boldsymbol{\theta})$, we denote $h(\boldsymbol{\theta})^{\otimes 0}$ for the function itself, $h(\boldsymbol{\theta})^{\otimes 1} = \nabla_{\boldsymbol{\theta}} h(\boldsymbol{\theta})$ for its gradient and $h(\boldsymbol{\theta})^{\otimes 2} = \nabla_{\boldsymbol{\theta}\boldsymbol{\theta}} h(\boldsymbol{\theta})$ for its Hessian. We also define

$$W_k^{(m)}(\boldsymbol{q}, \boldsymbol{x}, t; \boldsymbol{\theta}) = (\nu_k(\boldsymbol{q}, \boldsymbol{x}, t; \boldsymbol{\psi})\alpha_k(t; \boldsymbol{\eta}) \exp(\boldsymbol{\beta}_k^T \boldsymbol{x}))^{\otimes m}$$
$$S^{(m)}(t; \boldsymbol{\theta}) = \left(\sum_{j=1}^{n} \xi_j(t) \sum_{k=1}^{K} \alpha_k(t; \boldsymbol{\eta}) \exp(\boldsymbol{\beta}_k^T \boldsymbol{x}_j)\right)^{\otimes m}$$
$$\overline{S}^{(m)}(t; \boldsymbol{\theta}) = E\left(\frac{1}{n} \sum_{j=1}^{n} \xi_j(t) \sum_{k=1}^{K} \alpha_k(t; \boldsymbol{\eta}) \exp(\boldsymbol{\beta}_k^T \boldsymbol{x}_j)\right)^{\otimes m}$$


*danielnevo@gmail.com

Now, writing $\ell^{\star}_{Q2} = L^{\star}_{Q2}$ in a counting process formulation we have

$$\ell^{\star}_{Q2}(\boldsymbol{\theta}) = \sum_{k=1}^{K} \tilde{\ell}^{\star}_{k}(\boldsymbol{\theta}) + \tilde{\ell}^{\star\star}(\boldsymbol{\theta})$$

where

$$\tilde{\ell}^{\star}_{k}(\boldsymbol{\theta}) = \int_0^{\tau} \sum_{i=1}^{n} \Big[\log(W_k^{(0)}(\boldsymbol{q}_i, \boldsymbol{X}_i, t_i; \boldsymbol{\theta})) - \log S^{(0)}(t_i; \boldsymbol{\theta})\Big]\, dN^{o}_{ik}(t),$$

$$\tilde{\ell}^{\star\star}(\boldsymbol{\theta}) = \int_0^{\tau} \sum_{i=1}^{n} \left[\log\left(\sum_{m=1}^{K} W_m(\boldsymbol{q}_i, \boldsymbol{X}_i, t_i; \boldsymbol{\theta})\right) - \log S^{(0)}(t_i; \boldsymbol{\theta})\right] dN_{iu}(t),$$

$\tau$ is the study end-time, $N^{o}_{ik}(t) := \delta_i \mathbb{I}\{\tilde{T}_i \le t, Y_i = k, O_i = 1\}$ is the observed-cause-specific counting process of subject $i$ and $N_{iu}(t) := \delta_i \mathbb{I}\{\tilde{T}_i \le t, O_i = 0\}$ is the unobserved-cause event counting process of subject $i$. We also denote $N_{ik}(t) = \delta_i \mathbb{I}\{\tilde{T}_i \le t, Y_i = k\}$ for the cause-specific personal counting process and $N_{i\cdot} = \sum_{k=1}^{K} N_{ik}(t) = \sum_{k=1}^{K} N^{o}_{ik}(t) + N_{iu}(t)$ for the personal event counting process. See also Lu and Tsiatis [2005]. We can now define $\mathcal{F}_t := \sigma(\{\xi_i(s), \boldsymbol{X}_i(s), N^{o}_{ik}(s), N_{iu}(s), \boldsymbol{Q}_i(s), k = 1, ..., K, i = 1, ..., n, s \in [0, t]\})$ for the relevant filtration ($\boldsymbol{Q}_i(s)$ is defined arbitrarily whenever $N^{o}_{ik}(s) = N_{iu}(s) = 0$). We also denote $\mathcal{F} = \mathcal{F}_{\tau}$.

The score function of $\ell^{\star}_{Q2}(\boldsymbol{\theta})$ is

$$\boldsymbol{U}^{\star}(\boldsymbol{\theta}) = \ell^{\star}_{Q2}(\boldsymbol{\theta})^{\otimes 1} = \sum_{k=1}^{K} \boldsymbol{U}^{\star}_{k}(\boldsymbol{\theta}) + \boldsymbol{U}^{\star\star}(\boldsymbol{\theta}), \tag{A.1}$$

with

$$\frac{1}{n}\boldsymbol{U}^{\star}_{k}(\boldsymbol{\theta}) = \int_0^{\tau} \frac{1}{n}\sum_{i=1}^{n} \frac{W_k^{(1)}(\boldsymbol{q}_i, \boldsymbol{X}_i, t_i; \boldsymbol{\theta})}{W_k^{(0)}(\boldsymbol{q}_i, \boldsymbol{X}_i, t_i; \boldsymbol{\theta})} dN^{o}_{ik}(t) - \int_0^{\tau} \frac{1}{n}\sum_{i=1}^{n} \frac{S^{(1)}(t_i; \boldsymbol{\theta})}{S^{(0)}(t_i; \boldsymbol{\theta})} dN^{o}_{ik}(t) \tag{A.2}$$

$$\frac{1}{n}\boldsymbol{U}^{\star\star}(\boldsymbol{\theta}) = \int_0^{\tau} \frac{1}{n}\sum_{i=1}^{n} \frac{\sum_{m=1}^{K} W_m^{(1)}(\boldsymbol{q}_i, \boldsymbol{X}_i, t_i; \boldsymbol{\theta})}{\sum_{m=1}^{K} W_m^{(0)}(\boldsymbol{q}_i, \boldsymbol{X}_i, t_i; \boldsymbol{\theta})} dN_{iu}(t) - \int_0^{\tau} \frac{1}{n}\sum_{i=1}^{n} \frac{S^{(1)}(t_i; \boldsymbol{\theta})}{S^{(0)}(t_i; \boldsymbol{\theta})} dN_{iu}(t) \tag{A.3}$$

The maximum partial likelihood estimator $\hat{\boldsymbol{\theta}}_n$ is then defined as the solution of $\boldsymbol{U}^{\star}(\boldsymbol{\theta})$. We assume the following standard regularity assumptions, which are similar to those given in the supplemental materials of a manuscript currently under review written by the part of the authors of this paper with other collaborators [Nevo et al., 2016]. That paper does not concern missing cause but other problems related to measurement error in misclassification of biomarkers in risk factor analysis of tumor data.

**(i)** For all $i$, the vector $\boldsymbol{X}_i(t)$ is a bounded, predictable process with respect to the history $\mathcal{F}$.

**(ii)** For all $k = 1, .., K$ and for all $t \in [0, \tau]$, $\alpha_k(t; \boldsymbol{\eta})$ is bounded and twice differentiable in $\boldsymbol{\eta}$ with continuous second derivatives.

**(iii)** $\bar{S}^{(m)}(t, \boldsymbol{\theta}_0), m = 0, 1, 2$ are continuous and bounded functions of $\boldsymbol{\theta}_0$ for all $t \in [0, \tau]$. Furthermore, $\bar{S}^{(0)}(t, \boldsymbol{\theta}_0)$ is bounded away of zero.

**(iv)** The normalized Hessian matrix $\boldsymbol{H}(\boldsymbol{\theta}) = n^{-1}\ell^{\star}_{Q2}(\boldsymbol{\theta})^{\otimes 2}$ is continuous in $\boldsymbol{\theta}_0$, and negative definite at $\boldsymbol{\theta}_0$ with probability that goes to one.

**(v)** For all $k$, $\nu_k^{(m)}(\boldsymbol{q}, \boldsymbol{x}, t; \boldsymbol{\psi})$ are continuous and bounded functions with respect to $\boldsymbol{\psi}$.

**(vi)** $\text{MAR}_{T,\boldsymbol{X},\boldsymbol{Q}}$. That is,
$P(O = 1|\delta = 1, Y = k, T = t, \boldsymbol{X} = \boldsymbol{x}, \boldsymbol{Q} = \boldsymbol{q}) = P(O = 1|\delta = 1, T = t, \boldsymbol{X} = \boldsymbol{x}, \boldsymbol{Q} = \boldsymbol{q})$

We can now move to the consistency and asymptotic normality proofs. Our proofs we present here can be seen as generalizations of the proofs in Nevo et al. [2016]. We note that the standard martingale-based approach for consistency and normality of the Cox model [Andersen and Gill, 1982] cannot be used here, because $\boldsymbol{Q}$ is not predictable with respect to the history at time $t$.

**Consistency** First we will show that $n^{-1}\boldsymbol{U}^{\star}(\boldsymbol{\theta})$ converges in probability to $u^{\star}(\boldsymbol{\theta})$, and that $u^{\star}$ satisfies $u^{\star}(\boldsymbol{\theta}_0) = 0$. We begin by rewriting (A.1) (divided by $n$) as

$$\frac{1}{n}\boldsymbol{U}^{\star}(\boldsymbol{\theta}) = \int_0^{\tau}\sum_{k=1}^{K}\frac{1}{n}\sum_{i=1}^{n}\frac{W_k^{(1)}(\boldsymbol{q}_i, \boldsymbol{X}_i, t_i; \boldsymbol{\theta})}{W_k^{(0)}(\boldsymbol{q}_i, \boldsymbol{X}_i, t_i; \boldsymbol{\theta})}dN^o_{ik}(t) + \int_0^{\tau}\frac{1}{n}\sum_{i=1}^{n}\frac{\sum_{m=1}^{K}W_m^{(1)}(\boldsymbol{q}_i, \boldsymbol{X}_i, t_i; \boldsymbol{\theta})}{\sum_{m=1}^{K}W_m^{(0)}(\boldsymbol{q}_i, \boldsymbol{X}_i, t_i; \boldsymbol{\theta})}dN_{iu}(t) \tag{A.4}$$
$$- \int_0^{\tau}\frac{1}{n}\sum_{i=1}^{n}\frac{S^{(1)}(t_i; \boldsymbol{\theta})}{S^{(0)}(t_i; \boldsymbol{\theta})}dN_{i\cdot}(t)$$

Next, note that for any $\mathcal{A} \in \Omega_q$ we have

$$P(\boldsymbol{Q}_i \in A|\mathcal{F}_{t^-}, dN^o_{ik}(t) = 1) = \int_{\mathcal{A}}\frac{\xi_i(t)\lambda_{01}(t)W_k^{(0)}(\boldsymbol{q}, \boldsymbol{x}_i, t; \boldsymbol{\theta})\pi(t, \boldsymbol{x}_i, \boldsymbol{q})}{P(dN^o_{ik}(t) = 1|\mathcal{F}_{t-})}d\boldsymbol{q},$$
$$P(\boldsymbol{Q}_i \in A|\mathcal{F}_{t^-}, dN_{iu}(t) = 1) = \int_{\mathcal{A}}\frac{\xi_i(t)\lambda_{01}(t)\left(\sum_{k=1}^{K}W_k^{(0)}(\boldsymbol{q}, \boldsymbol{x}_i, t; \boldsymbol{\theta})\right)\overline{\pi}(t, \boldsymbol{x}_i, \boldsymbol{q})}{P(dN_{iu}(t) = 1|\mathcal{F}_{t-})}d\boldsymbol{q}$$

Now, each of the terms inside the first integral in (A.4) converges to its expectation uniformly in $t$ and $k$. Evaluated at $\boldsymbol{\theta}_0$, this expectation equals to

$$\begin{aligned}
&E\left(\frac{1}{n}\sum_{i=1}^{n}\frac{W_k^{(1)}(\boldsymbol{q}_i, \boldsymbol{X}_i, t_i; \boldsymbol{\theta}_0)}{W_k^{(0)}(\boldsymbol{q}_i, \boldsymbol{X}_i, t_i; \boldsymbol{\theta}_0)}dN^o_{ik}(t)\right)\\
&= EE\left(\frac{1}{n}\sum_{i=1}^{n}\frac{W_k^{(1)}(\boldsymbol{q}_i, \boldsymbol{X}_i, t_i; \boldsymbol{\theta}_0)}{W_k^{(0)}(\boldsymbol{q}_i, \boldsymbol{X}_i, t_i; \boldsymbol{\theta}_0)}dN^o_{ik}(t)\middle|\mathcal{F}_{t^-}\right)\\
&= E\left[\frac{1}{n}\sum_{i=1}^{n}P(dN^o_{ik}(t) = 1|\mathcal{F}_{t^-})E\left(\frac{W_k^{(1)}(\boldsymbol{q}_i, \boldsymbol{X}_i, t_i; \boldsymbol{\theta}_0)}{W_k^{(0)}(\boldsymbol{q}_i, \boldsymbol{X}_i, t_i; \boldsymbol{\theta}_0)}\middle|\mathcal{F}_{t^-}, dN^o_{ik}(t) = 1\right)\right]\\
&= E\left[\frac{1}{n}\sum_{i=1}^{n}P(dN^o_{ik}(t) = 1|\mathcal{F}_{t^-})\int_{\Omega_{\boldsymbol{q}}}\frac{\xi_i(t)\lambda_{01}(t)W_k^{(1)}(\boldsymbol{q}, \boldsymbol{X}_i, t_i; \boldsymbol{\theta}_0)\pi(t, \boldsymbol{X}_i, \boldsymbol{q})}{P(dN^o_{ik}(t) = 1|\mathcal{F}_{t^-})}d\boldsymbol{q}\right]\\
&= \lambda_{01}(t)E\left[\frac{1}{n}\sum_{i=1}^{n}\xi_i(t)(\alpha_k(t; \boldsymbol{\eta}_0)\exp(\boldsymbol{\beta}_k^T\boldsymbol{X}_i))^{\otimes 1}\int_{\Omega_{\boldsymbol{q}}}\nu_k(\boldsymbol{q}, \boldsymbol{X}_i, t; \boldsymbol{\psi})\pi(t, \boldsymbol{X}_i, \boldsymbol{q})d\boldsymbol{q}\right].
\end{aligned}$$

Similarly, the term inside the second integral in (A.4) also converges, uniformly in $t$, to its expectation. Evaluated at $\boldsymbol{\theta}_0$, this expectation equals to

$$
\begin{aligned}
& E\left(\frac{1}{n}\sum_{i=1}^{n}\frac{\sum_{m=1}^{K}W_m^{(1)}(\boldsymbol{q}_i,\boldsymbol{X}_i,t_i;\boldsymbol{\theta}_0)}{\sum_{m=1}^{K}W_m^{(0)}(\boldsymbol{q}_i,\boldsymbol{X}_i,t_i;\boldsymbol{\theta}_0)}dN_{iu}(t)\right) \\
&= EE\left(\frac{1}{n}\sum_{i=1}^{n}\frac{1}{n}\sum_{i=1}^{n}\frac{\sum_{m=1}^{K}W_m^{(1)}(\boldsymbol{q}_i,\boldsymbol{X}_i,t_i;\boldsymbol{\theta}_0)}{\sum_{m=1}^{K}W_m^{(0)}(\boldsymbol{q}_i,\boldsymbol{X}_i,t_i;\boldsymbol{\theta}_0)}dN_{iu}(t)\middle|\mathcal{F}_{t^-}\right) \\
&= E\left[\frac{1}{n}\sum_{i=1}^{n}P(dN_{iu}(t)=1|\mathcal{F}_{t^-})E\left(\frac{\sum_{m=1}^{K}W_m^{(1)}(\boldsymbol{q}_i,\boldsymbol{X}_i,t_i;\boldsymbol{\theta}_0)}{\sum_{m=1}^{K}W_m^{(0)}(\boldsymbol{q}_i,\boldsymbol{X}_i,t_i;\boldsymbol{\theta}_0)}\middle|\mathcal{F}_{t^-},dN_{iu}(t)=1\right)\right] \\
&= E\left[\frac{1}{n}\sum_{i=1}^{n}P(dN_{iu}(t)=1|\mathcal{F}_{t^-})\int_{\Omega_{\boldsymbol{q}}}\frac{\xi_i(t)\lambda_{01}(t)W_k^{(1)}(\boldsymbol{q},\boldsymbol{X}_i,t_i;\boldsymbol{\theta}_0)\overline{\pi}(t,\boldsymbol{X}_i,\boldsymbol{q})}{P(dN_{iu}(t)=1|\mathcal{F}_{t^-})}d\boldsymbol{q}\right] \\
&= \lambda_{01}(t)E\left[\frac{1}{n}\sum_{i=1}^{n}\xi_i(t)\sum_{m=1}^{K}\left((\alpha_m(t;\boldsymbol{\eta}_0)\exp(\beta_m^T\boldsymbol{X}_i))^{\otimes 1}\int_{\Omega_{\boldsymbol{q}}}\nu_m(\boldsymbol{q},\boldsymbol{X}_i,t;\boldsymbol{\psi})\overline{\pi}(t,\boldsymbol{X}_i,\boldsymbol{q})d\boldsymbol{q}\right)\right].
\end{aligned}
$$

Therefore, and since $\overline{\pi}(t,\boldsymbol{X}_i,\boldsymbol{q})=1-\pi(t,\boldsymbol{X}_i,\boldsymbol{q})$, the sum of the first two terms in (A.4) converges to (when evaluated at $\boldsymbol{\theta}_0$)

$$
\begin{aligned}
&\int_0^{\tau}\lambda_{01}(t)E\left[\frac{1}{n}\sum_{i=1}^{n}\xi_i(t)\sum_{k=1}^{K}\left((\alpha_k(t;\boldsymbol{\eta}_0)\exp(\beta_k^T\boldsymbol{X}_i))^{\otimes 1}\int_{\Omega_{\boldsymbol{q}}}\nu_k(\boldsymbol{q},\boldsymbol{X}_i,t;\boldsymbol{\psi})d\boldsymbol{q}\right)\right] \\
&\qquad = \int_0^{\tau}\lambda_{01}(t)\overline{S}^{(1)}(t;\boldsymbol{\theta}_0)
\end{aligned}
$$

since $\int_{\Omega_{\boldsymbol{q}}}\nu_k(\boldsymbol{q},\boldsymbol{x},t;\boldsymbol{\psi})d\boldsymbol{q}=1$ for all $k$.

Turning to the last term in (A.4), first note that by the weak law of the large numbers, and by the regularity assumptions outlined above $n^{-1}S^{(m)}(t_i;\boldsymbol{\theta}_0)$ converges in probability to $\bar{S}^{(m)}(t_i;\boldsymbol{\theta}_0)$ for $m=0,1,2$ and uniformly in $t$. It can be shown that

$$
\int_0^{\tau}\frac{1}{n}\sum_{i=1}^{n}\frac{S^{(1)}(t_i;\boldsymbol{\theta}_0)}{S^{(0)}(t_i;\boldsymbol{\theta}_0)}dN_{i\cdot}(t)=\int_0^{\tau}\frac{1}{n}\sum_{i=1}^{n}\frac{\bar{S}^{(1)}(t_i;\boldsymbol{\theta}_0)}{\bar{S}^{(0)}(t_i;\boldsymbol{\theta}_0)}dN_{i\cdot}(t)+o_p(1) \tag{A.5}
$$

Next, under $\text{MAR}_{T,\boldsymbol{X},\boldsymbol{Q}}$ $N_{i\cdot}(t)$ is a counting process with an intensity process

$$
\tilde{\lambda}_i(t)=\lambda_{01}(t)\xi_i(t)\sum_{k=1}^{K}\alpha_k(t;\boldsymbol{\eta}_0)\exp(\boldsymbol{\beta}_k^T\boldsymbol{x}_i)
$$

and the usual decomposition $dN_{i\cdot}(t)=\tilde{\lambda}_i(t)+dM_i(t)$ holds with $M_i(t)$ being a mean-zero martingale. Now, the fraction inside the integral in the leading term in the right hand side of

(A.5) converges to its expectation, evaluated at $\boldsymbol{\theta}_0$, this expectation equals to

$$
\begin{aligned}
E\left(\frac{\bar{S}^{(1)}(t_i;\boldsymbol{\theta}_0)}{\bar{S}^{(0)}(t_i;\boldsymbol{\theta}_0)}\frac{1}{n}\sum_{i=1}^{n} dN_{i\cdot}(t)\right) &= EE\left(\frac{\bar{S}^{(1)}(t_i;\boldsymbol{\theta}_0)}{\bar{S}^{(0)}(t_i;\boldsymbol{\theta}_0)}\frac{1}{n}\sum_{i=1}^{n} dN_{i\cdot}(t)\middle|\,\mathcal{F}_{t^-}\right)\\
&= E\left(\frac{\bar{S}^{(1)}(t_i;\boldsymbol{\theta}_0)}{\bar{S}^{(0)}(t_i;\boldsymbol{\theta}_0)}\frac{1}{n}\sum_{i=1}^{n} E(dN_{i\cdot}(t)|\mathcal{F}_{t^-})\right) + EE\left(\frac{\bar{S}^{(1)}(t_i;\boldsymbol{\theta}_0)}{\bar{S}^{(0)}(t_i;\boldsymbol{\theta}_0)}d\bar{M}_{\cdot}(t)\middle|\,\mathcal{F}_{t^-}\right)\\
&= \frac{\bar{S}^{(1)}(t_i;\boldsymbol{\theta}_0)}{\bar{S}^{(0)}(t_i;\boldsymbol{\theta}_0)}E\left(\frac{1}{n}\sum_{i=1}^{n}\tilde{\lambda}_i(t)\right) + EE\left(\frac{\bar{S}^{(1)}(t_i;\boldsymbol{\theta}_0)}{\bar{S}^{(0)}(t_i;\boldsymbol{\theta}_0)}d\bar{M}_{\cdot}(t)\middle|\,\mathcal{F}_{t^-}\right)\\
&= \lambda_{01}(t)\bar{S}^{(1)}(t_i;\boldsymbol{\theta}_0) + EE\left(\frac{\bar{S}^{(1)}(t_i;\boldsymbol{\theta}_0)}{\bar{S}^{(0)}(t_i;\boldsymbol{\theta}_0)}d\bar{M}_{\cdot}(t)\middle|\,\mathcal{F}_{t^-}\right)
\end{aligned}
$$

where $\bar{M}_{\cdot}(t) = n^{-1}\sum_{i=1}^{n} M_{i\cdot}(t)$ is a mean zero martingale as well. Now, taking the integral over $t$ of the above expression, the integral of the second term is zero, since $\bar{S}^{(1)}(t_i;\boldsymbol{\theta}_0)/\bar{S}^{(0)}(t_i;\boldsymbol{\theta}_0)$ is a predictable process with respect to $\mathcal{F}$ and $\bar{M}_{\cdot}(t)$ is a mean zero martingale. We get that

$$
\int_0^{\tau}\frac{1}{n}\sum_{i=1}^{n}\frac{S^{(1)}(t_i;\boldsymbol{\theta}_0)}{S^{(0)}(t_i;\boldsymbol{\theta}_0)}dN_{i\cdot}(t) \xrightarrow{p} \int_0^{\tau}\lambda_{01}(t)\overline{S}^{(1)}(t;\boldsymbol{\theta}_0)
$$

which cancels out the two first terms in (A.4). We get that $n^{-1}\boldsymbol{U}^{\star}(\boldsymbol{\theta})$ converges in probability to $u^{\star}(\boldsymbol{\theta})$, and that $u^{\star}(\boldsymbol{\theta}_0) = 0$. Consistency of $\hat{\boldsymbol{\theta}}$ follows from Foutz [1977].

**Normality** To establish normality, we follow the approach of Lin and Wei [1989]. We first show that $\sqrt{n}\boldsymbol{U}(\boldsymbol{\theta}_0)$ converges to a normally distributed random variable. As before, we have

$$
\boldsymbol{U}^{\star}(\boldsymbol{\theta}) = \sum_{k=1}^{K}\boldsymbol{U}_k^{\star}(\boldsymbol{\theta}) + \boldsymbol{U}^{\star\star}(\boldsymbol{\theta}).
$$

Now, define

$$
\boldsymbol{\zeta}_{ik}(\boldsymbol{\theta}) = \int_0^{\tau}\left[\frac{W_k^{(1)}(\boldsymbol{q}_i,\boldsymbol{X}_i,t;\boldsymbol{\theta})}{W_k^{(0)}(\boldsymbol{q}_i,\boldsymbol{X}_i,t;\boldsymbol{\theta})} - \frac{\overline{S}^{(1)}(t;\boldsymbol{\theta})}{\overline{S}^{(0)}(t;\boldsymbol{\theta})}\right]dN_{ik}^{o}(t)
$$

and for each $k$ we have

$$
\sqrt{n}\boldsymbol{U}_k^{\star}(\boldsymbol{\theta}) = \sqrt{n}\left[\frac{1}{n}\sum_{i=1}^{n}\boldsymbol{\zeta}_{ik}(\boldsymbol{\theta}) - \int_0^{\tau}\left(\frac{S^{(1)}(t;\boldsymbol{\theta})}{S^{(0)}(t;\boldsymbol{\theta})} - \frac{\overline{S}^{(1)}(t;\boldsymbol{\theta})}{\overline{S}^{(0)}(t;\boldsymbol{\theta})}\right)\frac{1}{n}\sum_{i=1}^{n}dN_{ik}^{o}(t)\right]
$$

Let $\boldsymbol{s}(t,\eta) = \frac{\overline{S}^{(1)}(t;\boldsymbol{\theta})}{\overline{S}^{(0)}(t;\boldsymbol{\theta})}$. Under the standard regularity conditions outlined above, we have for all $t \in [0,\tau]$,

$$
\frac{S^{(1)}(t;\boldsymbol{\theta})}{S^{(0)}(t;\boldsymbol{\theta})} - \boldsymbol{s}(t,\boldsymbol{\theta}) = \frac{S(t;\boldsymbol{\theta})^{(1)} - \boldsymbol{s}(t,\boldsymbol{\theta})S^{(0)}(t;\boldsymbol{\theta})}{\overline{S}^{(0)}(t;\boldsymbol{\theta})} + o_p(1).
$$

Let $\mathcal{N}_k^{o}(t) = E(N_{ik}^{o}(t))$. It can be shown that

$$
\int_0^{\tau}\frac{S^{(1)}(t;\boldsymbol{\theta}) - \boldsymbol{s}(t,\boldsymbol{\theta})S^{(0)}(t;\boldsymbol{\theta})}{\overline{S}^{(0)}(t;\boldsymbol{\theta})}\frac{1}{\sqrt{n}}\sum_{i=1}^{n}dN_{ik}^{o}(t) = \int_0^{\tau}\frac{S^{(1)}(t;\boldsymbol{\theta}) - \boldsymbol{s}(t,\boldsymbol{\theta})S^{(0)}(t;\boldsymbol{\theta})}{\overline{S}^{(0)}(t;\boldsymbol{\theta})}d\mathcal{N}_k^{o}(t) + o_p(1)
$$

since $\sqrt{n}(d\overline{N}_k(t) - d\mathcal{N}_k^o(t))$ converges to a mean zero Gaussian process. Now, let

$$a_i(t;\boldsymbol{\theta}) = \sum_{k=1}^{K} \alpha_k(t;\boldsymbol{\eta}) \exp(\boldsymbol{\beta}_k^T \boldsymbol{X}_i),$$

and we may write $\sqrt{n}\boldsymbol{U}_k^\star(\boldsymbol{\theta}) = n^{-1/2}\sum_{i=1}^n \boldsymbol{Z}_{ik} + o_p(1)$ where

$$\boldsymbol{Z}_{ik}(\boldsymbol{\theta}) = \boldsymbol{\zeta}_{ik}(\boldsymbol{\theta}) - \int_0^\tau \frac{a_i(t;\boldsymbol{\theta})^{\otimes 1} - a_i(t;\boldsymbol{\theta})\boldsymbol{s}(t,\boldsymbol{\theta})}{\overline{S}^{(0)}(t;\boldsymbol{\theta})} d\mathcal{N}_k^o(t).$$

Similar arguments can be applied to show that $\sqrt{n}\boldsymbol{U}^{\star\star}(\boldsymbol{\theta}) = n^{-1/2}\sum_{i=1}^n \boldsymbol{Z}_i^\star + o_p(1)$, where

$$\boldsymbol{Z}_i^\star(\boldsymbol{\theta}) = \boldsymbol{\zeta}_i^\star(\boldsymbol{\theta}) - \int_0^\tau \frac{a_i(\boldsymbol{\theta};t)^{\otimes 1} - a_i(t;\boldsymbol{\theta})\boldsymbol{s}(t,\boldsymbol{\theta})}{\overline{S}^{(0)}(t;\boldsymbol{\theta})} d\mathcal{N}^\star(t),$$

where $\boldsymbol{\zeta}_i^\star$ and $\mathcal{N}^\star(t)$ are the appropriate analogues of $\boldsymbol{\zeta}_{ik}$ and $\mathcal{N}_k^o(t)$, respectively. Now, let $\boldsymbol{R}_i(\boldsymbol{\theta}) = \sum_{k=1}^K \boldsymbol{Z}_{ik}(\boldsymbol{\theta}) + \boldsymbol{Z}_i^\star(\boldsymbol{\theta})$. Assuming $K$ is fixed, we get that the distribution of $\sqrt{n}\boldsymbol{U}^\star(\boldsymbol{\theta}_0)$ is asymptotically the same as the asymptotic distribution of $n^{-1/2}\sum_{i=1}^n \boldsymbol{R}_i(\boldsymbol{\theta}_0)$ which is, by a multivariate central limit theorem for iid random variables, is multivariate normal with a covariance matrix that can be consistently estimated from the data by $n^{-1}\sum_{i=1}^n \hat{\boldsymbol{R}}_i(\hat{\boldsymbol{\theta}})\hat{\boldsymbol{R}}_i(\hat{\boldsymbol{\theta}})^T$, where $\hat{\boldsymbol{R}}_i(\boldsymbol{\theta})$ is obtained by replacing expectations with sample means in $\boldsymbol{R}_i(\boldsymbol{\theta})$.

Finally, by a standard Taylor expansion argument we get that $\sqrt{n}(\hat{\boldsymbol{\theta}} - \boldsymbol{\theta}_0)$ converges to a normally distributed random variable with mean zero and covariance matrix that can be consistently estimated by

$$(n\boldsymbol{H}(\hat{\boldsymbol{\theta}}))^{-1}\left(\frac{1}{n}\sum_{i=1}^n \hat{\boldsymbol{R}}_i(\hat{\boldsymbol{\theta}})\hat{\boldsymbol{R}}_i(\hat{\boldsymbol{\theta}})^T\right)(n\boldsymbol{H}(\hat{\boldsymbol{\theta}}))^{-1}.$$

# Web Appendix B: Logistic regression model under MAR$_{\boldsymbol{Q}}$ and NMAR when $\gamma_t = \gamma_x = 0$

The goal of this appendix is to give a formal motivation for why both our methods are expected to be valid for the first simulation design we considered in the main text, i.e., under MAR$_{\boldsymbol{Q}}$. The simulation study results were given in Table 1 of the main text. We denote here

$$\psi_k = \text{logit}(P(Q=1|Y=k)), \qquad k = 1,2 \tag{A.6}$$

with $\text{logit}(u) = \log(u/(1-u))$. For the simulation study, we took $\psi_1 = \text{logit}(0.25)$ and $\psi_2 = \text{logit}(0.5)$. Now, consider the parametrization (with some abuse of notation comparing to the main text)

$$\text{logit}\,P(O=1|Q=q) = \gamma_q, \tag{A.7}$$

for $q = 0,1$. We want to show that given equations (A.6) and (A.7), the logistic regression model

$$\text{logit}\,P(O=1|Y=y) = \nu_y, \tag{A.8}$$

for $y = 1, 2$ also holds. The proof is rater strategist-forward. By the total law of probability we have

$$\nu_1 = \text{logit}[P(O = 1|Q = 1)P(Q = 1|Y = 1) + P(O = 1|Q = 0)P(Q = 0|Y = 1)]$$
$$= \text{logit}[\text{expit}(\gamma_1)\,\text{expit}(\psi_1) + \text{expit}(\gamma_0)(1 - \text{expit}(\psi_1))]$$

and similarly

$$\nu_2 = \text{logit}[\text{expit}(\gamma_1)\,\text{expit}(\psi_2) + \text{expit}(\gamma_0)(1 - \text{expit}(\psi_2))].$$

We note that with a more general logistic regression model for the missing, that includes additional covariates such as $\boldsymbol{X}$ and $T$, $\text{MAR}_{T,\boldsymbol{X},\boldsymbol{Q}}$ and NMAR do not necessarily hold simultaneously.

# Web Appendix C: Further simulation results

We first present here, in Web Table 1, the results under the same design as in Table 2 of the main text, but for sample size of 1,000. The standard deviation was larger for all methods. The methods based on $L^\star_Q$ and $L^\star_Y$ show larger bias for the small sample size, however they remain better than the GR and CCA methods.

Web Table 1: Simulation results for complete case analysis (CCA), estimating equation approach (GR) and our methods: $L^\star_Q$ and $L^\star_Y$ under $\text{MAR}_{T,\boldsymbol{X},\boldsymbol{Q}}$ and NMAR, as described in the main text. True values for the parameters were $\beta_1 = 0.223 = \log(1.25)$ and $\beta_2 = 0.916 = \log(2.5)$. Sample size for each simulation iteration was 1,000.

| | $(e^{\gamma_q}, e^{\gamma_y})$ | %Missing | | $\beta_1$ (true value 0.223) | | | | $\beta_2$ (true value 0.916) | | | |
|---|---|---|---|---|---|---|---|---|---|---|---|
| | | | | CCA | $L^\star_Q$ | $L^\star_Y$ | GR | CCA | $L^\star_Q$ | $L^\star_Y$ | GR |
| $\text{MAR}_{T,\boldsymbol{X},\boldsymbol{Q}}$ | 1,0 | 49.5% | Bias(%) | 125.26 | -2.13 | 2.21 | -2.14 | 34.67 | -0.33 | -0.59 | -3.22 |
| | | | SD | 0.28 | 0.25 | 0.25 | 0.25 | 0.22 | 0.16 | 0.17 | 0.18 |
| | 1.25,0 | 47.2% | Bias(%) | 111.14 | -7.05 | -0.62 | -9.58 | 31.72 | -0.32 | 1.04 | -2.92 |
| | | | SD | 0.27 | 0.23 | 0.23 | 0.24 | 0.21 | 0.17 | 0.18 | 0.19 |
| | 1.75,0 | 44.1% | Bias(%) | 105.38 | -6.99 | 2.79 | -14.11 | 28.47 | -0.36 | 2.16 | -4.74 |
| | | | SD | 0.26 | 0.23 | 0.22 | 0.24 | 0.20 | 0.17 | 0.18 | 0.18 |
| | 2.5,0 | 41.0% | Bias(%) | 96.99 | -6.37 | 6.59 | -17.93 | 24.10 | -0.85 | 3.00 | -6.65 |
| | | | SD | 0.26 | 0.22 | 0.21 | 0.23 | 0.19 | 0.16 | 0.18 | 0.18 |
| | 5,0 | 36.1% | Bias(%) | 84.23 | -4.99 | 16.24 | -24.55 | 19.14 | -0.74 | 4.37 | -9.28 |
| | | | SD | 0.25 | 0.22 | 0.20 | 0.24 | 0.19 | 0.17 | 0.19 | 0.18 |
| NMAR | 0,1 | 49.5% | Bias(%) | 123.10 | -2.94 | 2.71 | -2.07 | 33.03 | -0.80 | -0.81 | -3.76 |
| | | | SD | 0.28 | 0.24 | 0.24 | 0.24 | 0.23 | 0.17 | 0.18 | 0.19 |
| | 0,1.25 | 46.1% | Bias(%) | 121.02 | 0.94 | 9.08 | -0.10 | 29.32 | -1.94 | 0.19 | -4.38 |
| | | | SD | 0.28 | 0.25 | 0.24 | 0.25 | 0.21 | 0.16 | 0.18 | 0.18 |
| | 0,1.75 | 41.0% | Bias(%) | 103.70 | -9.57 | -1.32 | -18.40 | 23.91 | -4.90 | -0.24 | -9.22 |
| | | | SD | 0.28 | 0.24 | 0.23 | 0.25 | 0.20 | 0.16 | 0.17 | 0.18 |
| | 0,2.5 | 36.2% | Bias(%) | 103.59 | -1.42 | 6.26 | -18.48 | 18.32 | -6.89 | 0.02 | -13.27 |
| | | | SD | 0.28 | 0.25 | 0.23 | 0.25 | 0.19 | 0.16 | 0.18 | 0.18 |
| | 0,5 | 28.7% | Bias(%) | 96.34 | 5.48 | 9.64 | -26.11 | 9.38 | -10.72 | -1.40 | -22.26 |
| | | | SD | 0.28 | 0.26 | 0.23 | 0.27 | 0.17 | 0.14 | 0.16 | 0.17 |

We also considered the robustness of the $L^\star_Q$ method for misspecification of the baseline hazard. We considered $\text{MAR}_{T,\boldsymbol{X},\boldsymbol{Q}}$ with all parameters being the same as in the main simulation study. Let $\{A_1, ..., A_5\} = \{(0, 18], (18, 36], ..., (72, 90]\}$ be a partition of the time axis into five equal length intervals. We compared between $\beta_1$ and $\beta_2$ estimates obtained from maximizing $L^\star_Q$ when correctly specifying the baseline hazard ratio $\alpha_2(t; \eta_1, \eta_2) = \eta_1 t^{\eta_2}$ and when taking the baseline hazard ratio to be a piecewise constant. That is, when assuming $\alpha_2(t; \boldsymbol{\eta}) = \overline{\eta}_j$ where $j$ is the index of the interval $t$ belongs to, i.e., $t \in A_j$. $\overline{\eta}_1, ..., \overline{\eta}_5$ were estimated as part of the

data. However, the true baseline hazard ratio was $\alpha_2(t;\eta_1,\eta_2) = \eta_1 t^{\eta_2}$. The results presented in Web Table 2 suggest that taking piecewise constant baseline hazard ratio does not result in an increase of the bias.

Web Table 2: Relative bias and standard deviations for estimates obtained from $L^\star_Q$ when baseline hazard ratio $\alpha_2$ was correctly specified and when taking piecewise constant function for it. True values for the parameters were $\beta_1 = 0.223 = \log(1.25)$ and $\beta_2 = 0.916 = \log(2.5)$. Sample size for each simulation iteration was 1,000. The truth was $\text{MAR}_{T,\boldsymbol{X},\boldsymbol{Q}}$.

| $e^{\gamma_q}$ | %Missing | | $\beta_1$ (true value 0.223) | | $\beta_2$ (true value 0.916) | |
|---|---|---|---|---|---|---|
| | | | $L^\star_Q$–correct | $L^\star_Q$–piecewise | $L^\star_Q$–correct | $L^\star_Q$–piecewise |
| 1.00 | 49.5% | Bias(%) | -3.59 | -1.82 | -1.08 | -1.27 |
| | | SD | 0.24 | 0.24 | 0.17 | 0.17 |
| 1.25 | 47.2% | Bias(%) | -7.28 | -5.23 | -0.08 | -0.30 |
| | | SD | 0.24 | 0.24 | 0.17 | 0.17 |
| 1.75 | 44.1% | Bias(%) | -2.79 | -0.62 | -0.15 | -0.39 |
| | | SD | 0.22 | 0.23 | 0.16 | 0.16 |
| 2.50 | 41.0% | Bias(%) | -4.06 | -2.78 | 0.34 | 0.18 |
| | | SD | 0.23 | 0.23 | 0.17 | 0.17 |
| 5.00 | 36.1% | Bias(%) | -5.87 | -4.34 | 0.19 | 0.01 |
| | | SD | 0.24 | 0.24 | 0.17 | 0.17 |

# Web Appendix D: Preliminary analysis of missingness pattern

We present in this web appendix preliminary results regrading the missing pattern. Recall that one cannot exclude NMAR based on the data. However, we can explore logistic regression models under $\text{MAR}_{T,\boldsymbol{X},\boldsymbol{Q}}$ , $\pi(t,\boldsymbol{x},q) = \text{expit}(\gamma_0 + \gamma_t t + \boldsymbol{\gamma}^T_{\boldsymbol{x}}\boldsymbol{x} + \gamma_q q)$, where the more restrictive $\text{MAR}_{T,\boldsymbol{X}}$ assumption holds if this model is correct and $\gamma_q = 0$. We also remind the reader that our method is valid regardless of which of these two assumptions are correct. The analysis described here concerned CRC cases only (as opposed to censored observations). Following the main text, we have 1844 cases, of which 598 with known MSI status. Let $O$ be the indicator of observing the MSI status. We fitted logistic regression model for $O$ given the risk factors described in the main text, the time of CRC diagnosis and the location (proximal or non-proximal). We included a linear term for effect of diagnosis time, and, alternatively, as a binary variable with cutoff point at age 75.

Since data had been collected for a few decades, and measurement tools and regulations were not fixed over this period, we included in the model a random intercept for the questionnaire cycle. In all models we have considered, the variance of this random effect was significantly larger than zero.

We considered backwards elimination based on BIC, and alternatively based on $p$-values. When we used $p$-values, a model with significant variables only (at significance level$<$ 0.1) includes the random intercept, the time of the diagnosis (regardless of its form) and the tumor location. When we used BIC as our criterion, the optimal model was a model with tumor location and aforementioned random effect only. The results suggest that tumors with proximal location are less likely to have missing MSI status. Furthermore, missing MSI status is more likely for older age of diagnosis. These results suggest that tumor location plays a role in the missing mechanism and that a method based on $L^\star_Q$ is likely to be more appropriate.

## Web Appendix E: Stratified analysis

In section 5 of the main text, we implemented a stratified version of $L_Q^\star$, where stratification is done with respect to the questionnaire cycle to allow for calender-time changes in the baseline hazard ratios. Let $s = 1, ..., S$ be the strata and let $\alpha_{sk}(t;\boldsymbol{\eta}) = \lambda_{0sk}(t)/\lambda_{0s1}(t)$ be the baseline hazard ratio function for stratum $s$ and subtype $k$. $\lambda_{0s}(t)$, the baseline hazard ratio in in stratum $s$ is left unspecified. Let $s_i$ be the stratum of subject $i$. The modification of $L_{Q2}^\star$ given by Equation (8) in the main text is

$$L_{Q2}^\star(\boldsymbol{\beta},\boldsymbol{\eta},\boldsymbol{\psi}) = \prod_{s=1}^{S}\prod_{i=1}^{n}\left\{\left[\frac{\nu_{y_i}(\boldsymbol{q},\boldsymbol{x},t;\boldsymbol{\psi})\alpha_{sy_i}(t_i;\boldsymbol{\eta})\exp(\boldsymbol{\beta}_{y_i}^T\boldsymbol{x}_i)}{\sum_{\{j:s_j=s\}}\xi_j(t_i)\sum_{m=1}^{K}\alpha_{sm}(t_i;\boldsymbol{\eta})\exp(\boldsymbol{\beta}_m^T\boldsymbol{x}_j)}\right]^{I\{\delta_i=O_i=1,s_i=s\}}\right.$$
$$\left.\times\left[\frac{\sum_{k=1}^{K}\nu_k(\boldsymbol{q},\boldsymbol{x},t;\boldsymbol{\psi})\alpha_{sk}(t_i;\boldsymbol{\eta})\exp(\boldsymbol{\beta}_k^T\boldsymbol{x}_i)}{\sum_{\{j:s_j=s\}}\xi_j(t_i)\sum_{m=1}^{K}\alpha_{sm}(t_i;\boldsymbol{\eta})\exp(\boldsymbol{\beta}_m^T\boldsymbol{x}_j)}\right]^{I\{\delta_i=1,O_i=0,s_i=s\}}\right\}.$$

In the CRC example described in the main text, we had two subtypes and we took the baseline hazard ratios to be constant in each strata $\alpha_{2s}(t;\eta) = \eta_s$. Recall that by definition $\alpha_{2s}(t;\eta) = 1$ for all $s$ and $t$.

## References


Per Kragh Andersen and Richard D Gill. Cox's regression model for counting processes: a large sample study. *The annals of statistics*, pages 1100–1120, 1982.

Robert V Foutz. On the unique consistent solution to the likelihood equations. *Journal of the American Statistical Association*, 72(357):147–148, 1977.

Danyu Y Lin and Lee-Jen Wei. The robust inference for the cox proportional hazards model. *Journal of the American Statistical Association*, 84(408):1074–1078, 1989.

Kaifeng Lu and Anastasios A Tsiatis. Comparison between two partial likelihood approaches for the competing risks model with missing cause of failure. *Lifetime Data Analysis*, 11(1): 29–40, 2005.

Daniel Nevo, David Zucker, Rulla M. Tamimi, and Molin Wang. Accounting for measurement error in biomarker data and misclassification of subtypes in the analysis of tumor data. *under review*, 2016.
